# Supplementary material for: Pre-processing Image using Brightening, CLAHE and RETINEX
Source: arXiv:2003.10822 source file (2020-03-22)
Supplement: Supplementary file 1 [file Appendix.pdf]

Appendix A:

| | Original image | Without pre-processing | Ground Truth | Brightening | Retinex | CLAHE | Brightening + Retinex | Retinex + Brightening | Brightening + CLAHE | CLAHE + Brightening | Retinex + CLAHE | CLAHE + Retinex | Brightening + Retinex + CLAHE | Brightening + CLAHE + Retinex | Retinex + Brightening + CLAHE | Retinex + CLAHE + Brightening | CLAHE + Brightening + Retinex | CLAHE + Retinex + Brightening |
|---|---|---|---|---|---|---|---|---|---|---|---|---|---|---|---|---|---|---|
| IMAGE 0 | | | | | | | | | | | | | | | | | | |
| i0_crop_0 | | 1893 | | 2037 | 552 | 2532 | 0 | 516 | 2517 | 2433 | 2019 | 900 | 198 | 492 | 2112 | 2016 | 0 | 921 |
| | 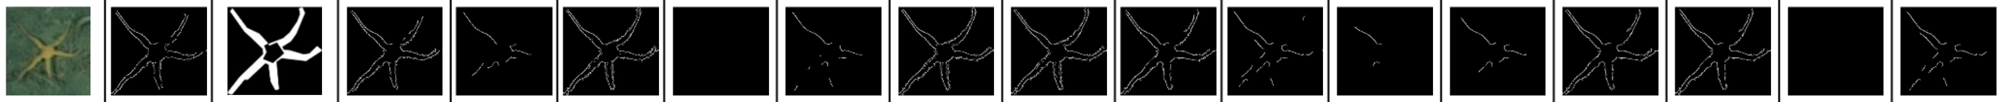 | | | | | | | | | | | | | | | | | |
| i0_crop_1 | | 2067 | | 2127 | 1917 | 2142 | 0 | 1764 | 2094 | 2139 | 2130 | 1590 | 1530 | 1188 | 2133 | 2124 | 657 | 1569 |
| | 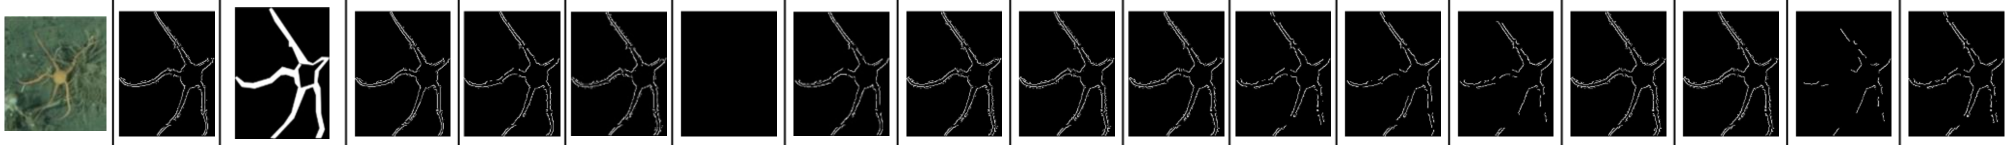 | | | | | | | | | | | | | | | | | |
| i0_crop_2 | | 2208 | | 2241 | 864 | 2670 | 0 | 858 | 2643 | 2649 | 2298 | 1194 | 498 | 591 | 2238 | 2322 | 0 | 1275 |
| | 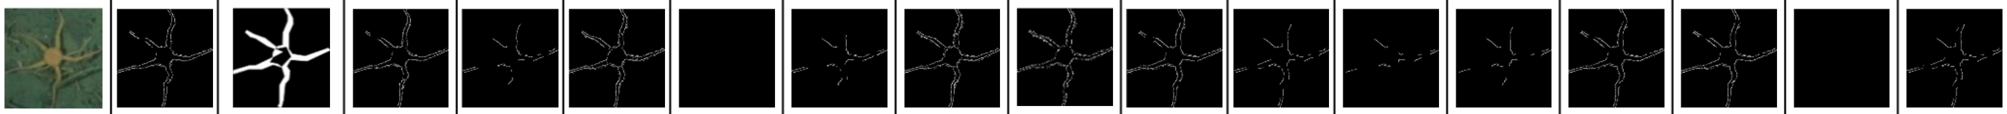 | | | | | | | | | | | | | | | | | |
| i0_crop_3 | | 3768 | | 3828 | 2790 | 3966 | 0 | 2973 | 4053 | 4014 | 3780 | 2961 | 2544 | 2325 | 3696 | 3720 | 1599 | 2940 |
| | 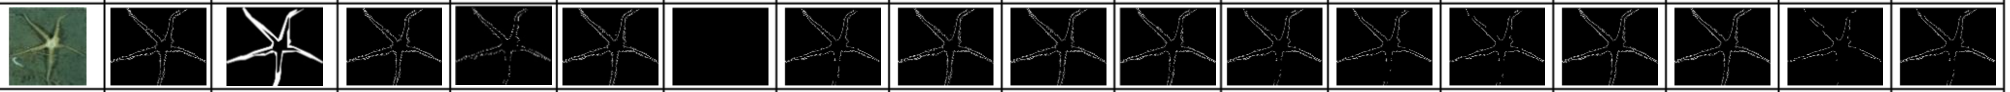 | | | | | | | | | | | | | | | | | |
| i0_crop_4 | | 2367 | | 2388 | 2118 | 2877 | 0 | 2151 | 2838 | 2844 | 2589 | 1986 | 1665 | 1497 | 2526 | 2670 | 738 | 2010 |
| | 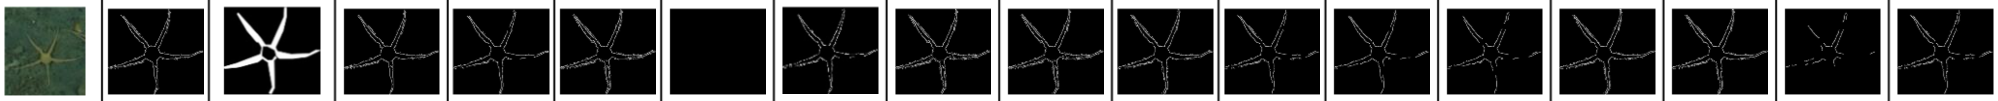 | | | | | | | | | | | | | | | | | |
| i0_crop_5 | | 1662 | | 1737 | 789 | 1842 | 0 | 738 | 1917 | 1851 | 1626 | 753 | 504 | 519 | 1602 | 1602 | 48 | 672 |
| | 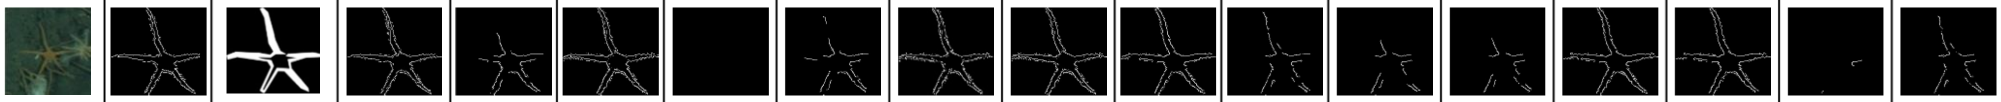 | | | | | | | | | | | | | | | | | |

| | Original image | Without pre-processing | Ground Truth | Brightening | Retinex | CLAHE | Brightening + Retinex | Retinex + Brightening | Brightening + CLAHE | CLAHE + Brightening | Retinex + CLAHE | CLAHE + Retinex | Brightening + Retinex + CLAHE | Brightening + CLAHE + Retinex | Retinex + Brightening + CLAHE | Retinex + CLAHE + Brightening | CLAHE + Brightening + Retinex | CLAHE + Retinex + Brightening |
|---|---|---|---|---|---|---|---|---|---|---|---|---|---|---|---|---|---|---|
| IMAGE 1 | | | | | | | | | | | | | | | | | | |
| i1_crop_0 | | 1863 | | 1905 | 933 | 2142 | 0 | 801 | 2067 | 2127 | 1842 | 966 | 633 | 831 | 1884 | 1899 | 300 | 954 |
| | 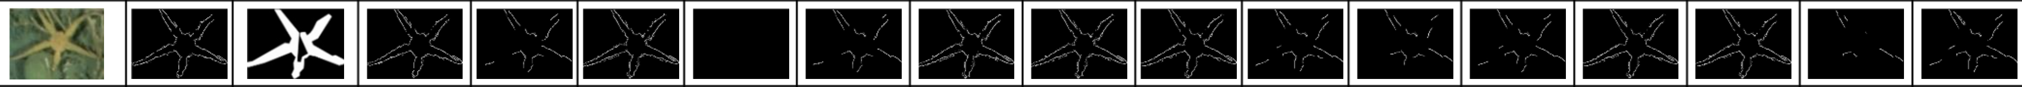 | | | | | | | | | | | | | | | | | |
| i1_crop_1 | | 483 | | 537 | 219 | 681 | 0 | 288 | 771 | 744 | 513 | 297 | 162 | 210 | 558 | 543 | 93 | 258 |
| | 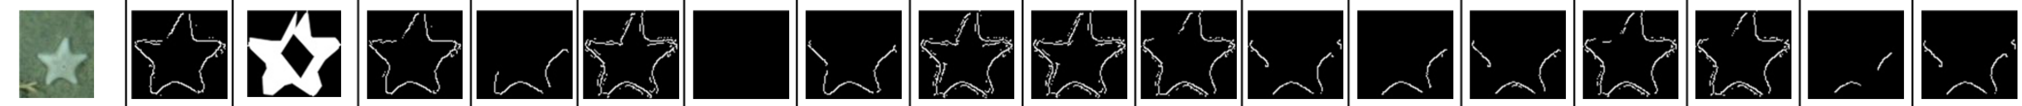 | | | | | | | | | | | | | | | | | |
| i1_crop_2 | | 1644 | | 1779 | 291 | 2103 | 0 | 252 | 2139 | 2151 | 1779 | 423 | 96 | 297 | 1800 | 1854 | 0 | 408 |
| | 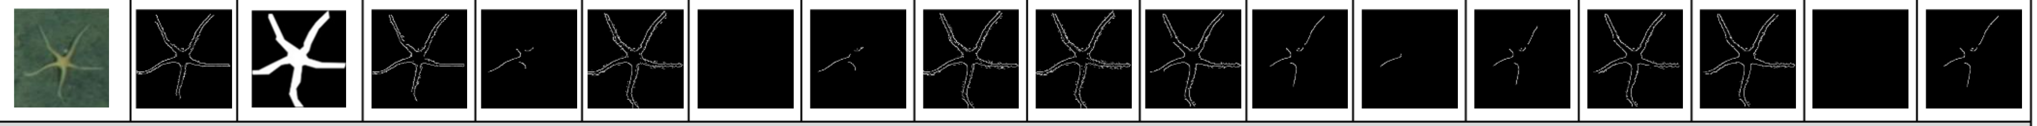 | | | | | | | | | | | | | | | | | |
| IMAGE 5 | | | | | | | | | | | | | | | | | | |
| i5_crop_0 | | 1290 | | 1233 | 1305 | 1554 | 0 | 1239 | 1467 | 1509 | 1425 | 951 | 1161 | 411 | 1434 | 1383 | 354 | 1065 |
| | 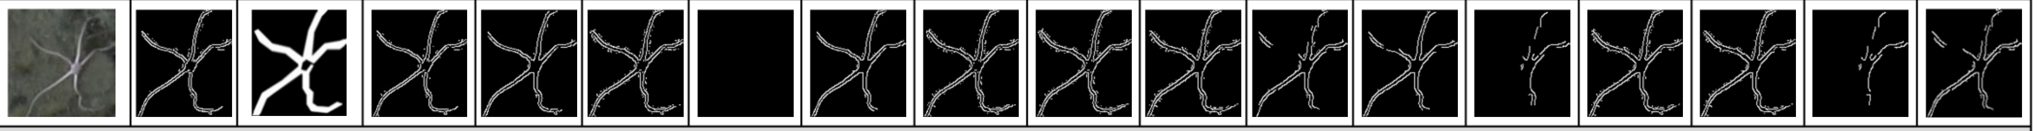 | | | | | | | | | | | | | | | | | |
| IMAGE 7 | | | | | | | | | | | | | | | | | | |
| i7_crop_0 | | 576 | | 495 | 138 | 645 | 69 | 138 | 750 | 675 | 615 | 312 | 204 | 225 | 573 | 624 | 159 | 279 |
| | 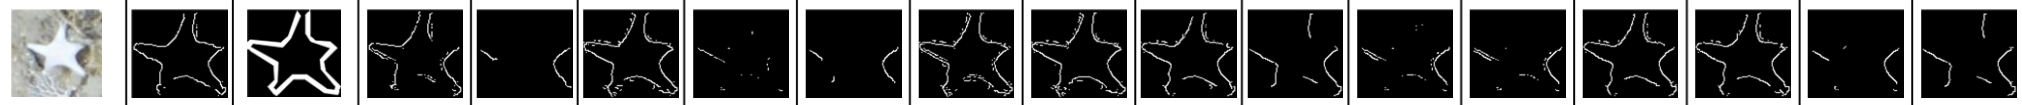 | | | | | | | | | | | | | | | | | |
| i7_crop_1 | | 1362 | | 1383 | 471 | 1845 | 0 | 459 | 1674 | 1854 | 1305 | 561 | 474 | 213 | 1347 | 1323 | 219 | 606 |
| | 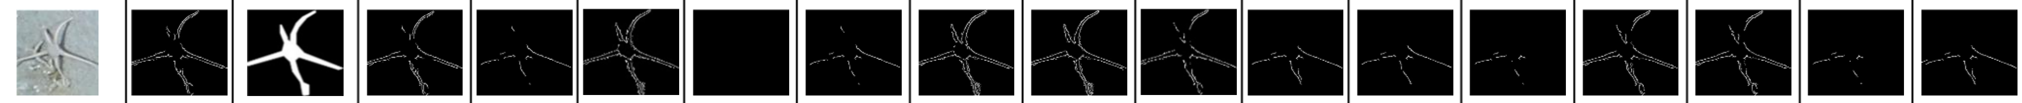 | | | | | | | | | | | | | | | | | |
| IMAGE 9 | | | | | | | | | | | | | | | | | | |
| i9_crop_0 | | 3702 | | 3501 | 0 | 13326 | 0 | 0 | 13488 | 14313 | 4665 | 1509 | 0 | 0 | 4698 | 4860 | 0 | 1362 |
| | 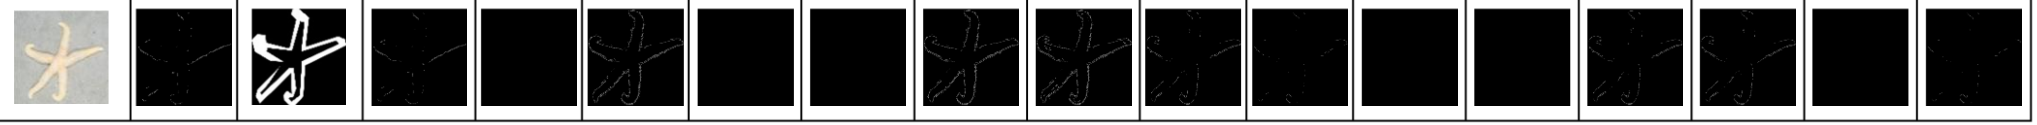 | | | | | | | | | | | | | | | | | |
